# Supplementary material for: Open Source Language Models Can Provide Feedback: Evaluating LLMs' Ability to Help Students Using GPT-4-As-A-Judge
Source: arXiv:2405.05253 source file (2024-05-08)
Supplement: Supplementary file 1 [file appendix.tex]

\appendix
\section{Appendix}

\input{appendix/a}

\input{appendix/b}
 
\input{appendix/c}
